# Supplementary material for: A-NeRF: Articulated Neural Radiance Fields for Learning Human Shape, Appearance, and Pose
Source: arXiv:2102.06199 source file (2021-10-29)
Supplement: Supplementary file 1 [file appendix_unused.tex]

\appendix
\section{Switching Times}

\section{Rodriges}
\SY{move the thing here to supp.}
 with the $4\times4$ local-to-world transformation matrix
\begin{align}
\jointtrans &= \prod_{j\in A(i)}\begin{bmatrix}
\exp(\smplbone_{(k,j)}) & \jointele_j \\ 
\mathbf{0} & 1
\end{bmatrix},\label{eq:joint-transform}
\end{align}
$\mathbf{0}=\left[0,0,0\right]$, $A(i)$ is the ordered set of the joint ancestors of $i$, and $\mathbf{\jointele}_i\in\jointelespace$ the joint location of $i$ at the rest pose. Since SPIN predicts $\mathbf{\jointele}_i\in\jointelespace$ for every image, we average the rest pose over all $k$ to obtain consistent bone length estimates.

The term $\exp(\subki{\smplbone})$ is the $3\times3$ rotation matrix computed using Rodrigues formula
\begin{equation}
    \exp(\subki{\smplbone})=\cI+\subki{\hat{\smplbone}}\sin\left(\subki{\smplbone}\right) + \subki{\hat{\smplbone}}^2\left(1-\cos(\norm{\subki{\smplbone}})\right),
\end{equation}
with, $\cI$ is the $3\times3$ identity matrix, $\subki{\hat{\smplbone}}$ is the $3\times 3$ skew matrix of the unit vector $\frac{\subki{\smplbone}}{\norm{\subki{\smplbone}}}$.
